# Supplementary material for: Hexagonal boron nitride as an ideal substrate for carbon nanotube photonics
Source: arXiv:2003.03054 ancillary file (2020-03-06)
Supplement: Supplementary file 1 [file hBN-SI.pdf]

**Supporting Information**

# Hexagonal boron nitride as an ideal substrate for carbon nanotube photonics

*Nan Fang,* [1,2] *Keigo Otsuka,* [1] *Akihiro Ishii,* [1,2] *Takashi Taniguchi,* [3] *Kenji Watanabe,* [3] *Kosuke Nagashio,* [4] *Yuichiro K. Kato* [1,2]

[1]Nanoscale Quantum Photonics Laboratory, RIKEN Cluster for Pioneering Research, Saitama 351-0198, Japan

[2]Quantum Optoelectronics Research Team, RIKEN Center for Advanced Photonics, Saitama 351-0198, Japan

[3]National Institute for Materials Science, Ibaraki 305-0044, Japan

[4]Department of Materials Engineering, The University of Tokyo, Tokyo 113-8656, Japan

**Supporting information**

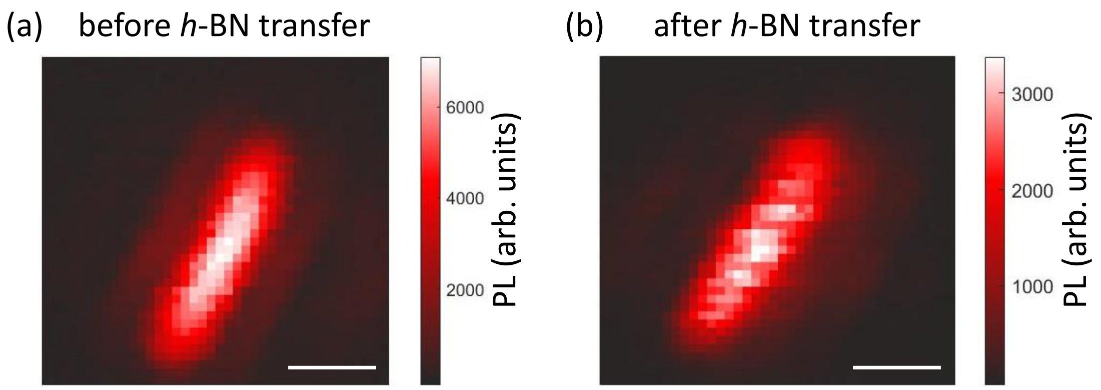


**Supplementary Figure S1.** (a, b) PL images for an air-suspended (9,7) carbon nanotube before and after the transfer of *h*-BN. Emission energies are 0.967 eV for (a) and 0.943 eV for (b), respectively. Scale bars are 1 μm. The shape of PL profile is almost unaffected by the *h*-BN transfer, indicating a homogenous interface between the CNT and *h*-BN.

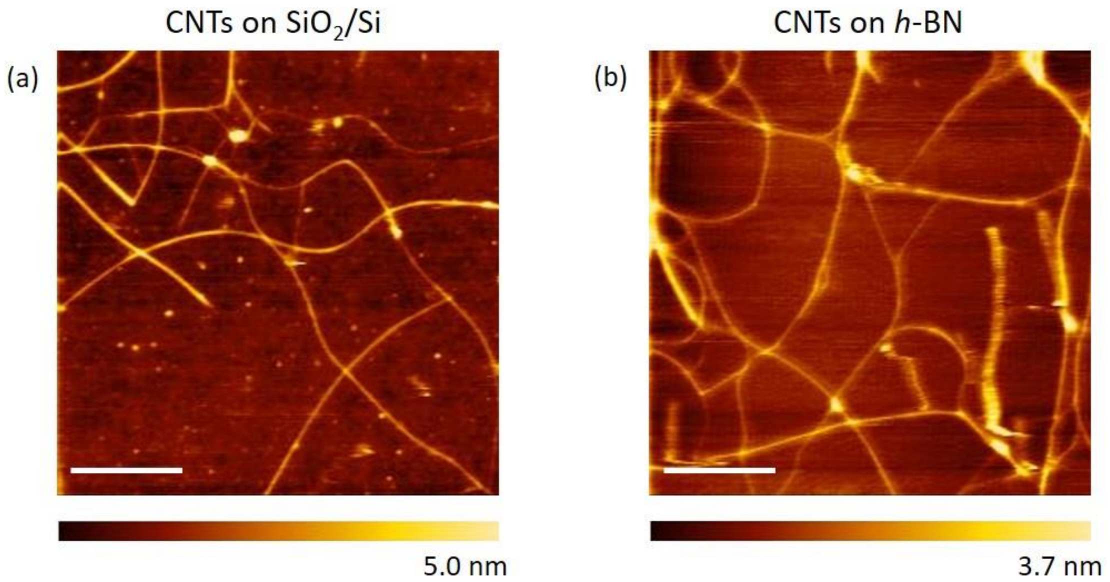


**Supplementary Figure S2.** AFM images of CNTs on (a) $SiO_2$/Si substrate and (b) *h*-BN substrate, respectively. Scale bars are 0.5 µm. It is clearly observed that the surface roughness of *h*-BN is smaller than that of the $SiO_2$/Si substrate. Many randomly oriented CNTs are firmly attached to both *h*-BN and the $SiO_2$/Si substrate without showing any loose ends or segments, and it can be seen that anthracene is fully sublimated.

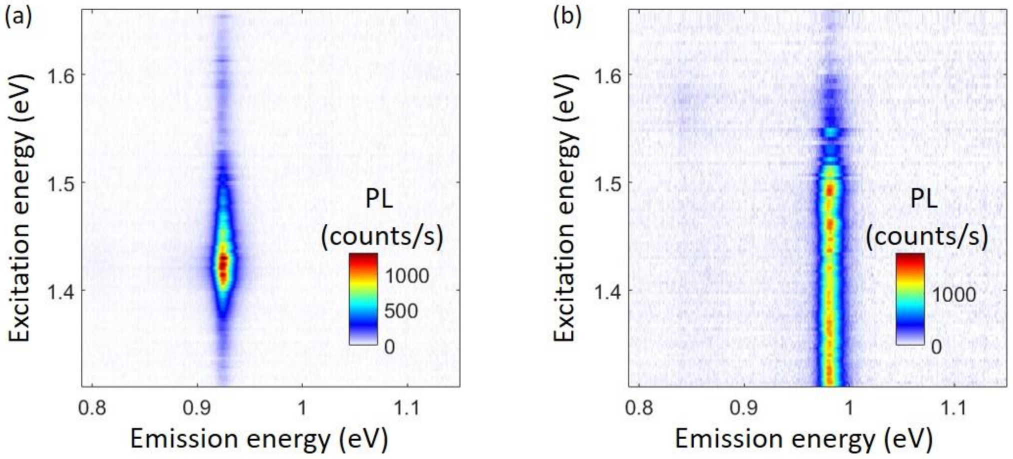


**Supplementary Figure S3.** (a) A typical PLE map from an individual CNT on *h*-BN. The clear $E_{11}$ and $E_{22}$ peaks indicate that photoluminescence comes from an individual tube. (b) An occasionally observed PLE map showing excitation spectra with smeared-out features. Such excitation spectra could result from exciton energy transfer between different types of tubes, which indicates bundling of CNTs. Both PLE maps are obtained at $P$ = 100 μW.
